# Supplementary material for: Accelerated Expansion of the Universe in Non-minimally Coupled Gravity
Source: arXiv:2301.02565 source file (2023-01-05)
Supplement: Supplementary file 1 [file AppendixA.tex]

% Appendix A

\chapter{Appendix Title Here} % Main appendix title

\label{AppendixA} % For referencing this appendix elsewhere, use \ref{AppendixA}

\lhead{Appendix A. \emph{Appendix Title Here}} % This is for the header on each page - perhaps a shortened title

Write your Appendix content here.
